# Supplementary material for: Knowledge Distillation Layer that Lets the Student Decide
Source: arXiv:2309.02843 source file (2023-09-06)
Supplement: Supplementary file 1 [file frontmatter.tex]

%\title{Supplementary Material for "Knowledge Distillation Layer that Lets the Student Decide"}
\def\etal{\emph{et al}\bmvaOneDot}
\runninghead{Gorgun \MakeLowercase{\etal}}{Supplementary Material}

\input{authors}
